# Supplementary material for: Low-Power IoT Communication Security: On the Performance of DTLS and TLS 1.3
Source: arXiv:2011.12035 source file (2020-12-10)
Supplement: Supplementary file 1 [file appendix.tex]

\section*{Appendix}
\begin{footnotesize}
In this appendix we describe our test setup in detail -- a cumbersome effort, in part due to the numerous possible configurations.

\paragraph*{CID}

We implemented and tested the new Connection ID functionality. For this purpose we compare the DTLS 1.3 CID implementation against the DTLS 1.2 CID implementation although the comparison is not entirely fair because the two versions offer slightly different properties.
\ \\
\paragraph*{TLS/DTLS Profiles}
To reduce the number of possible combinations we use the following profiles in our tests
(i) TLS 1.3 with PSK authentication and AES-128-CCM, 
(ii) TLS 1.3 with PSK authentication using AES-128-CCM and AES-256-CCM,
(iii) TLS 1.3 with ECDSA-ECDHE authentication using AES-128-CCM. The P256r1 curve was used for ECC-based crypto,
(iv) TLS 1.3 with ECDSA-ECDHE authentication using AES-256-CCM. The P512r1 curve was used for ECC-based crypto, 
(v) TLS 1.3 supporting all features implemented, including PSK and ECDSA-ECDHE authentication with AES-128-CCM and AES-256-CCM. Additionally, the 0-RTT mode, the backwards compatiblity mode, and the ticket extension was included. We do not include the library for parsing certificates in PEM format in the configuration nor the combination of ECDHE with PSK. We refer to this mode as the `full' configuration. 

The same profiles have been used with DTLS 1.3.
\ \\
\paragraph*{mbedTLS Configuration}

For the Mbed TLS stack the following configuration was used: 

\begin{itemize}

\item We use deterministic ECDSA (RFC 6979), as recommended in RFC 7925. The directive is MBEDTLS\_ECDSA\_DETERMINISTIC.

\item For the implementation of the preudo random number generator both a HMAC and block cipher in counter mode deterministic random bit generator (DRBG), defined in NIST SP 800-90A, were used. HMAC\_DRBG is utilized by the deterministic ECDSA mode while our application configures the CTR\_DRBG for use with the random number generator callback. Re-writing the application code to use a single DRBG would, however, be possible. The directives for these DRBGs are MBEDTLS\_HMAC\_DRBG\_C and MBEDTLS\_CTR\_DRBG\_C. 

\item We use the Server Name Indication (SNI) extension defined in RFC 6066, as recommended in RFC 7925. SNI allows a client to tell a server what FQDN it wants to contact. SNI has become popoular in the hosting environment where many virtual servers use a single IP address. It does, however, increase the size of the ClientHello message. We use the SNI extension only with public key crypto authentication. 

\item We only use ECC for asymmetric crypto and utilize various optimization techniques. First, fast modular reduction is enabled (MBEDTLS\_SSL\_ECP\_NIST\_OPTIM) and the technique is described in Appendix D.2 of FIPS 186-4. Next, we enable fixed point optimization to pre-compute points. This technique is enabled with the MBEDTLS\_SSL\_ECP\_FIXED\_POINT\_OPTIM pre-processor directive and described in~\cite{fixed-point}. Finally, we enable the sliding window technique described in~\cite{window}.We set the window size value to 7, which is the highest possible.  While all these techniques improve ECC runtime computations they require more RAM. 

\item For use with AES we opt for using less flash size at the expense of increased RAM utilization and degraded CPU performance. When MBEDTLS\_AES\_FEWER\_TABLES and MBEDTLS\_AES\_ROM\_TABLES are not declared then the RAM utilization is decreased by around 6 Kb (from 8.5 Kb to around 2.5 Kb).

\item For X.509 processing we enable MBEDTLS\_X509\_CHECK\_KEY\_USAGE for security reasons and set the MBEDTLS\_X509\_MAX\_INTERMEDIATE\_CA to one. 

\item For TLS 1.3 we limit the number of key shares sent in a ClientHello to one with the MBEDTLS\_SSL\_MAX\_KEY\_SHARES directive. Sending fewer key shares reduces the message size but may lead to additional handshake messages when the server does not support the group of the offered key share. Since IoT deployments are have a rather static setup we do not accept to see problems in practice. 

\end{itemize}

\end{footnotesize}
